# Supplementary material for: Screening Mixed-Metal Sn$_2$M(III)Ch$_2$X$_3$ Chalcohalides for Photovoltaic Applications
Source: arXiv:2306.17745 source file (2023-09-12)
Supplement: Supplementary file 2 [file suppinfo_sn2bch2x3.pdf]

# Screening Mixed-Metal $\text{Sn}_2\text{M(III)Ch}_2\text{X}_3$ Chalcohalides for Photovoltaic Applications

Pascal Henkel,<sup>†</sup> Jingrui Li,<sup>‡</sup> G. Krishnamurthy Grandhi,<sup>¶</sup> Paola Vivo,<sup>¶</sup> and Patrick  
Rinke\*,<sup>†</sup>

<sup>†</sup>*Department of Applied Physics, Aalto University, P.O.Box 11100, FI-00076 AALTO,  
Finland*

<sup>‡</sup>*Electronic Materials Research Laboratory, Key Laboratory of the Ministry of Education  
and International Center for Dielectric Research, School of Electronic Science and  
Engineering & International Joint Laboratory for Micro/Nano Manufacturing and  
Measurement Technology, Xi'an Jiaotong University, Xi'an 710049, China*

<sup>¶</sup>*Hybrid Solar Cells, Faculty of Engineering and Natural Sciences, Tampere University,  
P.O. Box 541, Tampere, FI, 33014, Finland*

E-mail: patrick.rinke@aalto.fi

# S1: Band structure of $\text{Sn}_2\text{InS}_2\text{Br}_3$

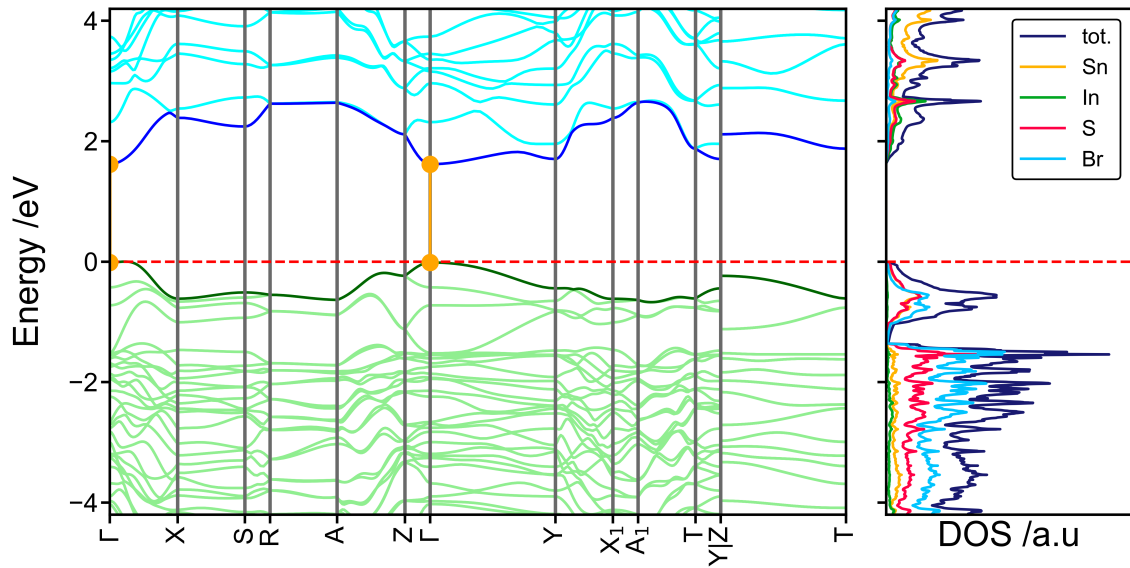

Figure 1: Bandstructure (left) and normalized density of states (right) for  $\text{Sn}_2\text{InS}_2\text{Br}_3$  for the  $Cmcm$  space group. Conduction bands are shown in green and valence bands in blue. The total and partial density of state per element are provided.

## S2: Lattice parameters, formation energies, fundamental and optical band gaps for $\text{Sn}_2\text{M(III)Ch}_2\text{X}_3$ materials

Table 1: Summary of the calculated lattice parameters ( $a$ ,  $b$ ,  $c$ ,  $a/c$ -ratio), as well as the formation energy  $E_{\text{form}}$  (related to the  $i$ -th elements) using PBEsol level of theory and the fundamental lowest direct band gap  $E_{\text{g, dir.}}$ , and for indirect  $\text{Sn}_2\text{M(III)Ch}_2\text{X}_3$  materials also the lowest indirect band gap ( $E_{\text{g, ind.}}$ ), as well as the optical band gap using HSE06+SOC level of theory. -/- marks that either the material has no indirect/no band gap at all or that no experimental values are available.  $\text{Sn}_2\text{M(III)Ch}_2\text{X}_3$  materials highlighted orange (direct) or gray (indirect) if their fundamental band gap is within the range of 0.7 eV to 2.0 eV.

| System                                | Group                   | lat. parameters |        |        |       | $E_{\text{form}}$ /eV Atom <sup>-1</sup> | $E_{\text{g, dir.}}$ | $E_{\text{g, ind.}}$ /eV | $E_{\text{g, opt.}}$ /eV |
|---------------------------------------|-------------------------|-----------------|--------|--------|-------|------------------------------------------|----------------------|--------------------------|--------------------------|
|                                       |                         | $a$ /Å          | $b$ /Å | $c$ /Å | $c/a$ |                                          |                      |                          |                          |
| $\text{Sn}_2\text{InS}_2\text{Cl}_3$  | <i>Cmcm</i>             | 4.23            | 14.12  | 14.3   | 3.38  | -726                                     | 1.305                | 1.251                    | 1.49                     |
|                                       | <i>Cmc2<sub>1</sub></i> | 3.94            | 14.22  | 15.0   | 3.81  | -772                                     | 1.834                | 1.692                    | 1.89                     |
|                                       | <i>P2<sub>1</sub>/c</i> | 6.27            | 16.19  | 7.88   | 1.26  | -779                                     | 2.433                | 2.037                    | 2.440                    |
| $\text{Sn}_2\text{InS}_2\text{Br}_3$  | <i>Cmcm</i>             | 4.22            | 14.80  | 14.50  | 3.44  | -650                                     | 1.617                | -/-                      | 1.977                    |
|                                       | <i>Cmc2<sub>1</sub></i> | 4.11            | 15.16  | 15.53  | 3.77  | -693                                     | 1.742                | -/-                      | 1.783                    |
|                                       | <i>P2<sub>1</sub>/c</i> | 6.36            | 16.55  | 8.07   | 1.27  | -690                                     | 1.985                | 1.616                    | 1.996                    |
| $\text{Sn}_2\text{InS}_2\text{I}_3$   | <i>Cmcm</i>             | 4.37            | 15.68  | 14.83  | 3.40  | -520                                     | 1.395                | -/-                      | 1.934                    |
|                                       | <i>Cmc2<sub>1</sub></i> | 4.06            | 14.13  | 19.25  | 4.75  | -519                                     | 1.120                | 0.598                    | 1.187                    |
|                                       | <i>P2<sub>1</sub>/c</i> | 7.66            | 16.56  | 8.41   | 1.1   | -565                                     | 2.278                | 2.102                    | 2.313                    |
| $\text{Sn}_2\text{InSe}_2\text{Cl}_3$ | <i>Cmcm</i>             | 4.13            | 14.94  | 14.9   | 3.60  | -718                                     | 0.661                | 0.597                    | 0.675                    |
|                                       | <i>Cmc2<sub>1</sub></i> | 4.08            | 14.09  | 16.02  | 3.93  | -767                                     | 1.046                | -/-                      | 1.684                    |
|                                       | <i>P2<sub>1</sub>/c</i> | 6.35            | 16.79  | 8.09   | 1.27  | -765                                     | 2.076                | 1.925                    | 2.088                    |
| $\text{Sn}_2\text{InSe}_2\text{Br}_3$ | <i>Cmcm</i>             | 4.42            | 14.54  | 15.01  | 3.40  | -651                                     | 1.105                | -/-                      | 1.477                    |
|                                       | <i>Cmc2<sub>1</sub></i> | 3.98            | 15.22  | 15.58  | 3.91  | -699                                     | 1.373                | 1.338                    | 1.396                    |
|                                       | <i>P2<sub>1</sub>/c</i> | 6.41            | 17.09  | 8.23   | 1.28  | -688                                     | 1.843                | 1.488                    | 1.855                    |
| $\text{Sn}_2\text{InSe}_2\text{I}_3$  | <i>Cmcm</i>             | 4.39            | 15.73  | 15.31  | 3.49  | -534                                     | 1.369                | 1.299                    | 1.397                    |
|                                       | <i>Cmc2<sub>1</sub></i> | 4.32            | 15.93  | 16.32  | 3.78  | -577                                     | 0.677                | -/-                      | 1.282                    |
|                                       | <i>P2<sub>1</sub>/c</i> | 7.41            | 17.62  | 8.5    | 1.15  | -567                                     | 1.947                | 1.785                    | 1.960                    |
| $\text{Sn}_2\text{InTe}_2\text{Cl}_3$ | <i>Cmcm</i>             | 4.19            | 12.25  | 18.4   | 4.39  | -542                                     | 0.558                | 0.455                    | 0.651                    |
|                                       | <i>Cmc2<sub>1</sub></i> | 4.16            | 13.24  | 17.21  | 4.13  | -639                                     | 0.915                | 0.804                    | 1.011                    |
|                                       | <i>P2<sub>1</sub>/c</i> | 6.53            | 17.82  | 8.58   | 1.32  | -610                                     | 1.594                | -/-                      | 1.713                    |
| $\text{Sn}_2\text{InTe}_2\text{Br}_3$ | <i>Cmcm</i>             | 4.28            | 12.34  | 18.41  | 4.30  | -488                                     | -/-                  | -/-                      | -/-                      |
|                                       | <i>Cmc2<sub>1</sub></i> | 4.31            | 14.70  | 16.90  | 3.92  | -559                                     | 0.531                | -/-                      | 0.786                    |
|                                       | <i>P2<sub>1</sub>/c</i> | 6.48            | 18.04  | 8.60   | 1.33  | -543                                     | 1.461                | -/-                      | 1.592                    |
| $\text{Sn}_2\text{InTe}_2\text{I}_3$  | <i>Cmcm</i>             | 4.56            | 15.6   | 16.26  | 3.57  | -425                                     | 1.089                | 0.994                    | 1.126                    |
|                                       | <i>Cmc2<sub>1</sub></i> | 4.3             | 15.34  | 16.92  | 3.94  | -460                                     | 0.867                | 0.802                    | 0.964                    |
|                                       | <i>P2<sub>1</sub>/c</i> | 6.58            | 18.87  | 8.74   | 1.33  | -438                                     | 1.109                | 1.083                    | 1.201                    |
| $\text{Sn}_2\text{SbS}_2\text{Cl}_3$  | <i>Cmcm</i>             | 4.08            | 12.63  | 15.88  | 3.89  | -649                                     | 1.679                | 1.611                    | 1.773                    |
|                                       | <i>Cmc2<sub>1</sub></i> | 4.01            | 13.81  | 16.0   | 3.99  | -655                                     | 1.242                | 1.056                    | 1.288                    |
|                                       | <i>P2<sub>1</sub>/c</i> | 6.96            | 16.05  | 8.08   | 1.16  | -702                                     | 2.451                | 2.170                    | 2.477                    |
| $\text{Sn}_2\text{SbS}_2\text{Br}_3$  | <i>Cmcm</i>             | 4.1             | 13.47  | 15.4   | 3.76  | -574                                     | 1.474                | 0.883                    | 1.527                    |
|                                       | <i>Cmc2<sub>1</sub></i> | 4.1             | 13.92  | 16.12  | 3.93  | -592                                     | 1.248                | 1.055                    | 1.344                    |
|                                       | <i>P2<sub>1</sub>/c</i> | 7.01            | 16.06  | 8.19   | 1.17  | -646                                     | 2.194                | 1.989                    | 2.294                    |
| $\text{Sn}_2\text{SbS}_2\text{I}_3$   | <i>Cmcm</i>             | 4.24            | 13.84  | 15.76  | 3.72  | -486                                     | 0.997                | 0.947                    | 1.547                    |
|                                       | <i>Cmc2<sub>1</sub></i> | 4.26            | 14.22  | 16.24  | 3.81  | -497                                     | 1.007                | -/-                      | 1.506                    |
|                                       | <i>P2<sub>1</sub>/c</i> | 7.25            | 16.24  | 8.47   | 1.17  | -555                                     | 1.762                | 1.686                    | 1.771                    |
|                                       | Exp. <sup>a</sup>       | 4.25            | 13.99  | 16.38  | 3.85  | -/-                                      | -/-                  | -/-                      | 1.41                     |
| $\text{Sn}_2\text{SbSe}_2\text{Cl}_3$ | <i>Cmcm</i>             | 4.16            | 12.48  | 16.92  | 4.07  | -646                                     | 1.411                | -/-                      | 1.816                    |
|                                       | <i>Cmc2<sub>1</sub></i> | 4.07            | 14.01  | 16.45  | 4.04  | -651                                     | 1.002                | -/-                      | 1.261                    |
|                                       | <i>P2<sub>1</sub>/c</i> | 7.06            | 17.98  | 8.06   | 1.14  | -692                                     | 2.181                | 1.839                    | 2.202                    |

| System                                | Group             | lat. parameters  |                  |                  |       | $E_{\text{form}} / \text{eV Atom}^{-1}$ | $E_{\text{g, dir.}}$ | $E_{\text{g, ind.}} / \text{eV}$ | $E_{\text{g, opt.}} / \text{eV}$ |
|---------------------------------------|-------------------|------------------|------------------|------------------|-------|-----------------------------------------|----------------------|----------------------------------|----------------------------------|
|                                       |                   | $a / \text{\AA}$ | $b / \text{\AA}$ | $c / \text{\AA}$ | $c/a$ |                                         |                      |                                  |                                  |
| $\text{Sn}_2\text{SbSe}_2\text{Br}_3$ | $Cmcm$            | 4.13             | 12.94            | 17.75            | 4.3   | -572                                    | 1.412                | 1.330                            | 1.504                            |
|                                       | $Cmc2_1$          | 4.16             | 14.22            | 16.73            | 4.03  | -586                                    | 0.941                | 0.891                            | 1.044                            |
|                                       | $P2_1/c$          | 7.1              | 17.16            | 8.29             | 1.17  | -631                                    | 2.028                | 1.642                            | 2.100                            |
| $\text{Sn}_2\text{SbSe}_2\text{I}_3$  | $Cmcm$            | 4.28             | 13.95            | 16.44            | 3.84  | -473                                    | 1.057                | 0.800                            | 1.056                            |
|                                       | $Cmc2_1$          | 4.31             | 14.50            | 16.91            | 3.93  | -493                                    | 0.962                | -/-                              | 1.640                            |
|                                       | $P2_1/c$          | 7.28             | 17.08            | 8.57             | 1.18  | -547                                    | 1.892                | 1.672                            | 1.983                            |
|                                       | Exp. <sup>b</sup> | 4.30             | 14.09            | 17.22            | 4.01  | -/-                                     | -/-                  | -/-                              | -/-                              |
| $\text{Sn}_2\text{SbTe}_2\text{Cl}_3$ | $Cmcm$            | 4.34             | 12.40            | 17.68            | 4.07  | -530                                    | 0.943                | 0.874                            | 0.997                            |
|                                       | $Cmc2_1$          | 4.34             | 12.39            | 17.70            | 4.08  | -523                                    | 0.950                | -/-                              | 1.370                            |
|                                       | $P2_1/c$          | 6.45             | 18.1             | 8.36             | 1.30  | -588                                    | 0.559                | 0.480                            | 0.653                            |
| $\text{Sn}_2\text{SbTe}_2\text{Br}_3$ | $Cmcm$            | 4.24             | 12.51            | 19.69            | 4.64  | -456                                    | 0.699                | 0.490                            | 0.763                            |
|                                       | $Cmc2_1$          | 4.27             | 14.66            | 17.39            | 4.07  | -456                                    | 1.027                | 0.980                            | 1.063                            |
|                                       | $P2_1/c$          | 6.59             | 18.5             | 8.42             | 1.28  | -518                                    | 0.545                | 0.245                            | 0.567                            |
| $\text{Sn}_2\text{SbTe}_2\text{I}_3$  | $Cmcm$            | 4.34             | 13.57            | 19.47            | 4.48  | -353                                    | 0.786                | 0.465                            | 0.795                            |
|                                       | $Cmc2_1$          | 4.28             | 14.31            | 18.73            | 4.37  | -358                                    | 0.376                | 0.186                            | 0.433                            |
|                                       | $P2_1/c$          | 7.02             | 18.82            | 8.67             | 1.24  | -412                                    | 0.852                | 0.021                            | 1.255                            |
| $\text{Sn}_2\text{BiS}_2\text{Cl}_3$  | $Cmcm$            | 3.99             | 13.91            | 16.02            | 4.02  | -714                                    | 1.535                | 0.986                            | 1.548                            |
|                                       | $Cmc2_1$          | 4.07             | 13.72            | 15.98            | 3.93  | -716                                    | 1.146                | 1.034                            | 1.169                            |
|                                       | $P2_1/c$          | 6.97             | 15.93            | 8.1              | 1.16  | -732                                    | 2.187                | 1.84                             | 2.191                            |
| $\text{Sn}_2\text{BiS}_2\text{Br}_3$  | $Cmcm$            | 4.11             | 13.42            | 15.68            | 3.81  | -650                                    | 1.343                | 0.956                            | 1.434                            |
|                                       | $Cmc2_1$          | 4.11             | 13.42            | 15.68            | 3.82  | -651                                    | 1.405                | 1.124                            | 1.504                            |
|                                       | $P2_1/c$          | 7.03             | 16.04            | 8.23             | 1.17  | -675                                    | 1.968                | 1.717                            | 2.065                            |
| $\text{Sn}_2\text{BiS}_2\text{I}_3$   | $Cmcm$            | 4.26             | 13.92            | 15.93            | 3.74  | -552                                    | 0.988                | -/-                              | 1.390                            |
|                                       | $Cmc2_1$          | 4.26             | 13.92            | 15.94            | 3.74  | -553                                    | 1.013                | -/-                              | 1.420                            |
|                                       | $P2_1/c$          | 7.3              | 16.23            | 8.52             | 1.17  | -583                                    | 1.606                | 1.490                            | 1.599                            |
|                                       | Exp. <sup>c</sup> | 4.29             | 14.12            | 16.41            | 3.83  | -/-                                     | -/-                  | -/-                              | 1.22                             |
| $\text{Sn}_2\text{BiSe}_2\text{Cl}_3$ | $Cmcm$            | 4.03             | 12.5             | 17.07            | 4.23  | -713                                    | 1.104                | 1.096                            | 1.124                            |
|                                       | $Cmc2_1$          | 4.13             | 13.98            | 16.46            | 3.99  | -708                                    | 0.902                | 0.714                            | 0.952                            |
|                                       | $P2_1/c$          | 6.41             | 17.23            | 8.22             | 1.28  | -731                                    | 1.196                | 1.076                            | 1.254                            |
| $\text{Sn}_2\text{BiSe}_2\text{Br}_3$ | $Cmcm$            | 4.13             | 13.02            | 17.29            | 4.19  | -635                                    | 0.965                | 0.666                            | 1.063                            |
|                                       | $Cmc2_1$          | 4.21             | 14.14            | 16.74            | 3.98  | -642                                    | 0.841                | 0.827                            | 0.853                            |
|                                       | $P2_1/c$          | 6.9              | 17.19            | 8.33             | 1.21  | -662                                    | 1.425                | 1.118                            | 1.452                            |
| $\text{Sn}_2\text{BiSe}_2\text{I}_3$  | $Cmcm$            | 4.31             | 13.99            | 16.62            | 3.86  | -538                                    | 1.048                | 0.769                            | 1.141                            |
|                                       | $Cmc2_1$          | 4.35             | 14.47            | 16.87            | 3.87  | -538                                    | 1.064                | 0.881                            | 1.162                            |
|                                       | $P2_1/c$          | 7.33             | 17.08            | 8.6              | 1.17  | -575                                    | 1.66                 | 1.474                            | 1.751                            |
| $\text{Sn}_2\text{BiTe}_2\text{Cl}_3$ | $Cmcm$            | 4.15             | 12.37            | 17.83            | 4.30  | -580                                    | 0.738                | -/-                              | 1.079                            |
|                                       | $Cmc2_1$          | 4.20             | 12.37            | 17.84            | 4.25  | -579                                    | 0.764                | 0.697                            | 0.863                            |
|                                       | $P2_1/c$          | 6.53             | 18.02            | 8.48             | 1.30  | -612                                    | 0.498                | 0.476                            | 0.579                            |
| $\text{Sn}_2\text{BiTe}_2\text{Br}_3$ | $Cmcm$            | 4.24             | 12.63            | 18.26            | 4.31  | -510                                    | 0.852                | 0.715                            | 0.854                            |
|                                       | $Cmc2_1$          | 4.24             | 12.64            | 18.27            | 4.31  | -510                                    | 0.854                | 0.718                            | 0.856                            |
|                                       | $P2_1/c$          | 6.68             | 18.39            | 8.53             | 1.28  | -542                                    | 0.597                | 0.440                            | 0.692                            |
| $\text{Sn}_2\text{BiTe}_2\text{I}_3$  | $Cmcm$            | 4.38             | 13.30            | 18.73            | 4.28  | -399                                    | -/-                  | -/-                              | -/-                              |
|                                       | $Cmc2_1$          | 4.48             | 14.90            | 17.96            | 4.05  | -407                                    | 0.610                | 0.582                            | 0.692                            |
|                                       | $P2_1/c$          | 7.12             | 18.67            | 8.75             | 1.23  | -439                                    | 0.890                | 0.256                            | 0.931                            |

<sup>a</sup> Lat. para. are taken from RT ( $T = 293 \text{ K}$ ) XRD meas. using  $\text{MoK}\alpha$  radiation<sup>1</sup> and band gap are taken from UV/vis absorption meas.<sup>2</sup>

<sup>b</sup> Lat. para. are taken from low-temp. ( $T = 173 \text{ K}$ ) XRD meas. using  $\text{MoK}\alpha$  radiation.<sup>1</sup>

<sup>c</sup> Lat. para. are taken from RT ( $T = 293 \text{ K}$ ) XRD meas. using  $\text{MoK}\alpha$  radiation and band gap are taken from UV/vis absorption meas.<sup>3</sup>

### S3: Formation energies for indirect $\text{Sn}_2\text{M(III)Ch}_2\text{X}_3$ materials

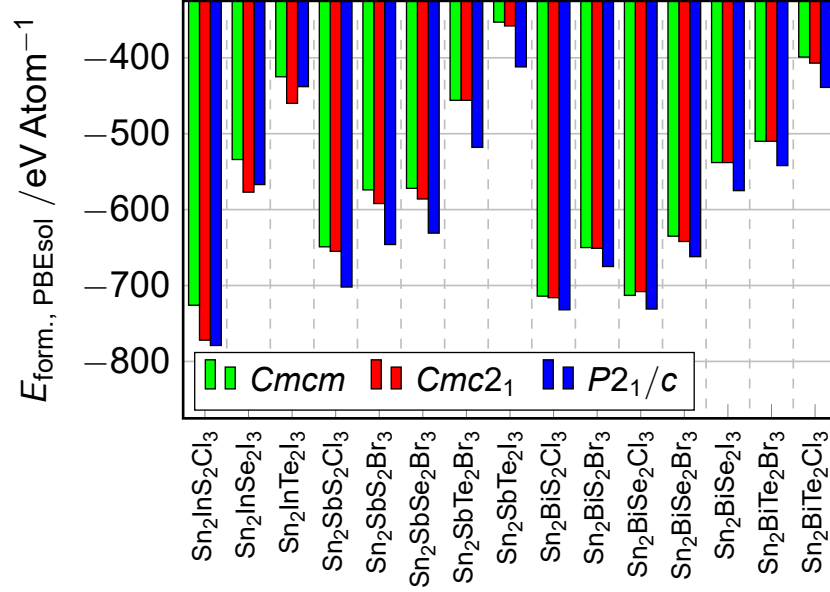

Figure 2: Formation energy (calculated with PBEsol) of the 15 indirect  $\text{Sn}_2\text{M(III)Ch}_2\text{X}_3$  compounds of interest for  $Cmc$  (green),  $Cmc2_1$  (red) and  $P2_1/c$  (blue) space groups.

S4: Band gaps for all identified direct and indirect  $\text{Sn}_2\text{M(III)Ch}_2\text{X}_3$  materials

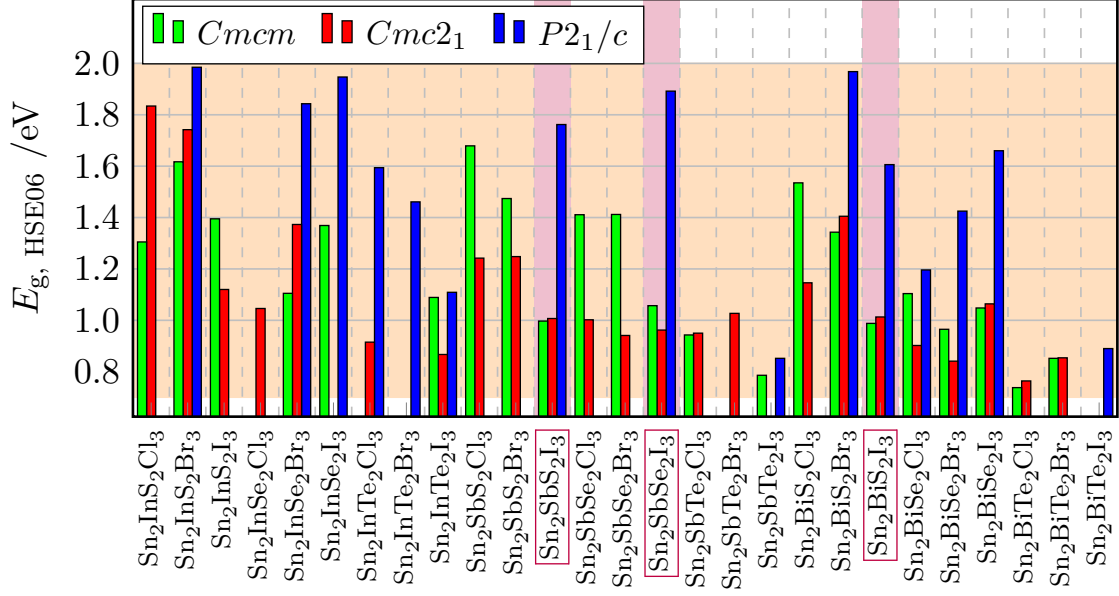

Figure 3: Direct band gaps (HSE06+SOC level of theory) for 12  $\text{Sn}_2\text{SbS}_2\text{I}_3$  materials of interest and energetically lowest direct band gaps (HSE06+SOC level of theory) for 15 indirect  $\text{Sn}_2\text{SbS}_2\text{I}_3$  materials of interest for  $Cmcm$  (green),  $Cmc2_1$  (red) and  $P2_1/c$  (blue) space groups. Three structures -  $\text{Sn}_2\text{SbS}_2\text{I}_3$ ,<sup>4</sup>  $\text{Sn}_2\text{SbSe}_2\text{I}_3$ ,<sup>1</sup> and  $\text{Sn}_2\text{BiS}_2\text{I}_3$ <sup>3</sup> - that are already known from the literature, are highlighted in purple.

## S5: $\text{Sn}_2\text{M(III)}_{1-a}\text{M(III)}'_a\text{Ch}_{2-b}\text{Ch}'_b\text{X}_{3-c}\text{X}'_c$ alloy compounds based on direct and indirect $\text{Sn}_2\text{M(III)}\text{Ch}_2\text{X}_3$ materials

Similar to the described approach of  $\text{Sn}_2\text{M(III)}_{1-a}\text{M(III)}'_a\text{Ch}_{2-b}\text{Ch}'_b\text{X}_{3-c}\text{X}'_c$  alloys with only  $\text{Sn}_2\text{M(III)}\text{Ch}_2\text{X}_3$  materials with direct gaps, we now consider also  $\text{Sn}_2\text{M(III)}\text{Ch}_2\text{X}_3$  materials with an indirect gaps. In this way, we obtain a considerably larger  $\text{Sn}_2\text{M(III)}_{1-a}\text{M(III)}'_a\text{Ch}_{2-b}\text{Ch}'_b\text{X}_{3-c}\text{X}'_c$  material space. The alloys we consider are composed either of two direct  $\text{Sn}_2\text{M(III)}\text{Ch}_2\text{X}_3$  materials, or of one direct and one indirect material, as well as of two indirect materials. For the indirect  $\text{Sn}_2\text{M(III)}\text{Ch}_2\text{X}_3$  compounds, we use the energetically lowest direct band gap, analogous to fig. 3 in the SI. By this we can identify a total of 81  $\text{Sn}_2\text{M(III)}_{1-a}\text{M(III)}'_a\text{Ch}_{2-b}\text{Ch}'_b\text{X}_{3-c}\text{X}'_c$  alloys [see fig. 4 in the SI], 69 of which are composed of at least one indirect  $\text{Sn}_2\text{M(III)}\text{Ch}_2\text{X}_3$  material.

The  $P2_1/c$  space group is no longer underrepresented and a homogenous distribution of the three space groups is obtained. Similar to their direct counterparts, the alloys within the  $Cmcm$  and  $Cmc2_1$  space group tend to have band gaps in the lower part of the spectra (about 1 eV), whereas  $P2_1/c$  alloys tend towards the upper region of the spectra (about 2 eV). These compounds open up the  $\text{Sn}_2\text{M(III)}_{1-a}\text{M(III)}'_a\text{Ch}_{2-b}\text{Ch}'_b\text{X}_{3-c}\text{X}'_c$  space and can also be considered for future band gap tuning. Thus, we assume that at least a part of compositions within this  $\text{Sn}_2\text{M(III)}_{1-a}\text{M(III)}'_a\text{Ch}_{2-b}\text{Ch}'_b\text{X}_{3-c}\text{X}'_c$  space may have a direct band gap that fulfils our materials design criterion, whereby these alloys might also be of interest.

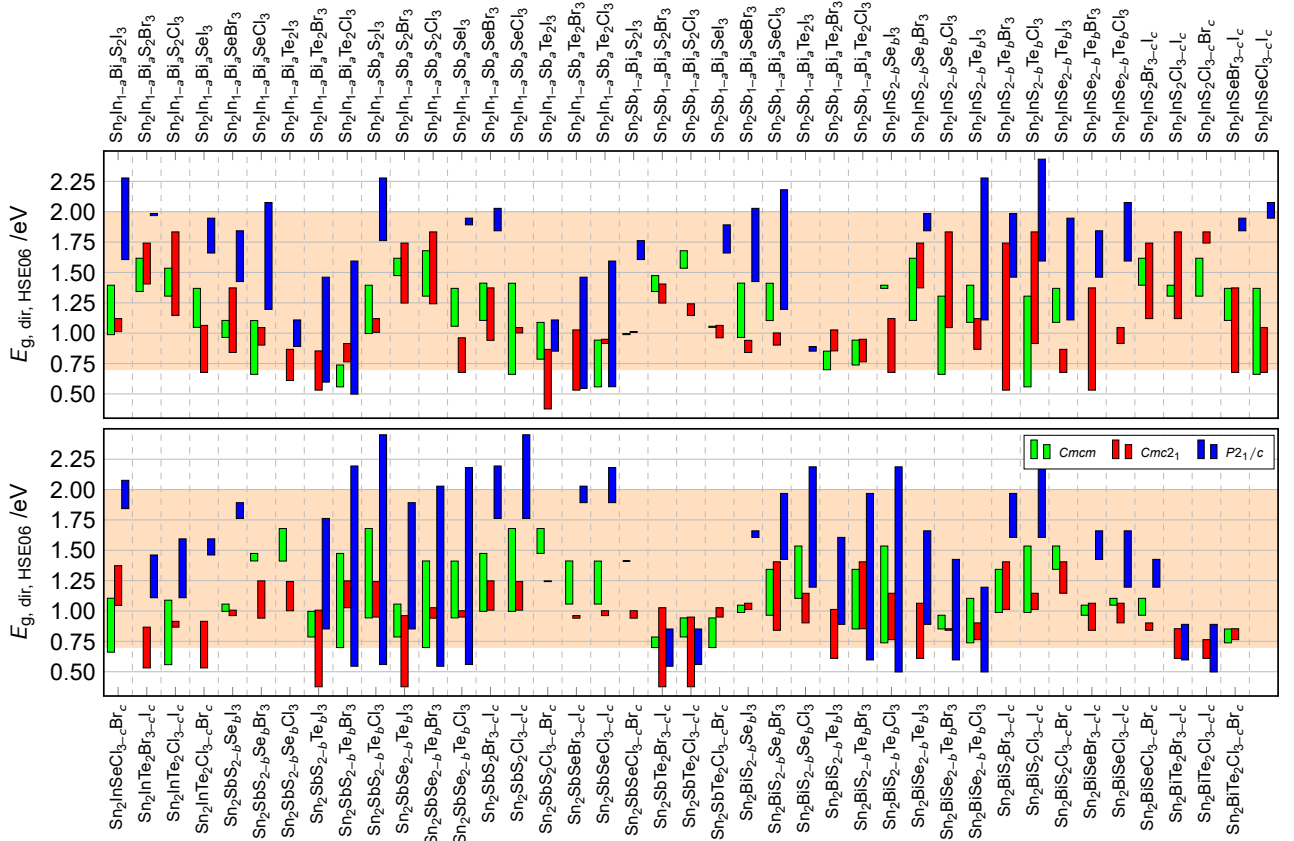

Figure 4: Band gap ranges (HSE06+SOC level of theory) for all 81  $Sn_2M(III)_{1-a}M(III)'_aCh_{2-b}Ch'_bX_{3-c}X'_c$  binary alloy compounds of interest based on direct an indirect  $Sn_2M(III)Ch_2X_3$  compounds for  $Cmcmm$  (green),  $Cmc2_1$  (red) and  $P2_1/c$  (blue) space groups.

## References

- (1) Ibanez, A.; Jumas, J.-C.; Olivier-Fourcade, J.; Philippot, E. Mise en évidence d'un désordre statistique dans les structures chalcogénoiodures d'étain et d'antimoine. *Journal of Solid State Chemistry* **1984**, *55*, 83–91.
- (2) Nie, R.; Lee, K. S.; Hu, M.; Paik, M. J.; Seok, S. I. Heteroleptic Tin-Antimony Sulfoiodide for Stable and Lead-free Solar Cells. *Matter* **2020**, *3*, 1701–1713.
- (3) Islam, S. M.; Malliakas, C. D.; Sarma, D.; Maloney, D. C.; Stoumpos, C. C.; Kontsevoi, O. Y.; Freeman, A. J.; Kanatzidis, M. G. Direct Gap Semiconductors  $\text{Pb}_2\text{BiS}_2\text{I}_3$ ,  $\text{Sn}_2\text{BiS}_2\text{I}_3$ , and  $\text{Sn}_2\text{BiSI}_5$ . *Chemistry of Materials* **2016**, *28*, 7332–7343.
- (4) Olivier-Fourcade, J.; Jumas, J. C.; Maurin, M.; Philippot, E. Mise en Évidence d'un Nouveau Sulfoiodure d'Étain et d'Antimoine  $\text{Sn}_2\text{SbS}_2\text{I}_3$ : Étude Structurale. *Zeitschrift für anorganische und allgemeine Chemie* **1980**, *468*, 91–98.
